# Supplementary material for: Principal Geodesic Analysis of Merge Trees (and Persistence Diagrams)
Source: arXiv:2207.10960 source file (2022-12-02)
Supplement: Supplementary file 5 [file appendixMetricsTable.tex]

\section{Metrics}

test
