# Supplementary material for: Principal Geodesic Analysis of Merge Trees (and Persistence Diagrams)
Source: arXiv:2207.10960 source file (2022-12-02)
Supplement: Supplementary file 9 [file appendix_VIS.tex]

\documentclass[review,journal]{vgtc}         % review (journal style)
%\documentclass[widereview]{vgtc}             % wide-spaced review
%\documentclass[preprint,journal]{vgtc}       % preprint (journal style)

%% Uncomment one of the lines above depending on where your paper is
%% in the conference process. ``review'' and ``widereview'' are for review
%% submission, ``preprint'' is for pre-publication, and the final version
%% doesn't use a specific qualifier.

%% Please use one of the ``review'' options in combination with the
%% assigned online id (see below) ONLY if your paper uses a double blind
%% review process. Some conferences, like IEEE Vis and InfoVis, have NOT
%% in the past.

%% Please note that the use of figures other than the optional teaser is not permitted on the first page
%% of the journal version.  Figures should begin on the second page and be
%% in CMYK or Grey scale format, otherwise, colour shifting may occur
%% during the printing process.  Papers submitted with figures other than the optional teaser on the
%% first page will be refused. Also, the teaser figure should only have the
%% width of the abstract as the template enforces it.

%% These few lines make a distinction between latex and pdflatex calls and they
%% bring in essential packages for graphics and font handling.
%% Note that due to the \DeclareGraphicsExtensions{} call it is no longer necessary
%% to provide the the path and extension of a graphics file:
%% \includegraphics{diamondrule} is completely sufficient.
%% 
\ifpdf%                                % if we use pdflatex
  \pdfoutput=1\relax                   % create PDFs from pdfLaTeX
  \pdfcompresslevel=9                  % PDF Compression
  \pdfoptionpdfminorversion=7          % create PDF 1.7
  \ExecuteOptions{pdftex}
  \usepackage{graphicx}                % allow us to embed graphics files
  \DeclareGraphicsExtensions{.pdf,.png,.jpg,.jpeg} % for pdflatex we expect .pdf, .png, or .jpg files
\else%                                 % else we use pure latex
  \ExecuteOptions{dvips}
  \usepackage{graphicx}                % allow us to embed graphics files
  \DeclareGraphicsExtensions{.eps}     % for pure latex we expect eps files
\fi%

%% it is recomended to use ``\autoref{sec:bla}'' instead of ``Fig.~\ref{sec:bla}''
\graphicspath{{figures/}{pictures/}{images/}{./}} % where to search for the images

\usepackage{microtype}                 % use micro-typography (slightly more compact, better to read)
\PassOptionsToPackage{warn}{textcomp}  % to address font issues with \textrightarrow
\usepackage{textcomp}                  % use better special symbols
\usepackage{mathptmx}                  % use matching math font
\usepackage{times}                     % we use Times as the main font
         % a nicer typewriter font
\usepackage{cite}                      % needed to automatically sort the references
\usepackage{tabu}                      % only used for the table example
\usepackage{booktabs}                  % only used for the table example

\usepackage{amsmath}                   % for math align env.
\usepackage{color}
\usepackage{mathptmx}
\usepackage{amssymb}
\usepackage{enumitem}
\usepackage{multicol}
\usepackage{anyfontsize}
\usepackage{amsmath}
\usepackage{algorithmic}
\usepackage{algorithm}
\usepackage{lipsum}  
\usepackage{esvect}
\DeclareMathAlphabet{\mathcal}{OMS}{cmsy}{m}{n}

%% We encourage the use of mathptmx for consistent usage of times font
%% throughout the proceedings. However, if you encounter conflicts
%% with other math-related packages, you may want to disable it.

%% In preprint mode you may define your own headline.
%\preprinttext{To appear in IEEE Transactions on Visualization and Computer Graphics.}

%% If you are submitting a paper to a conference for review with a double
%% blind reviewing process, please replace the value ``0'' below with your
%% OnlineID. Otherwise, you may safely leave it at ``0''.
\onlineid{1073}

%% declare the category of your paper, only shown in review mode
\vgtccategory{Research}
%% please declare the paper type of your paper to help reviewers, only shown in review mode
%% choices:
%% * algorithm/technique
%% * application/design study
%% * evaluation
%% * system
%% * theory/model
% \vgtcpapertype{Algorithm / Technique}

%% Paper title.
\title{Principal Geodesic Analysis of Merge Trees\\ (and Persistence Diagrams)\\-\\Appendix}

%% This is how authors are specified in the journal style

%% indicate IEEE Member or Student Member in form indicated below
\author{Mathieu Pont, and Julien Tierny}
\authorfooter{
%% insert punctuation at end of each item
\item
 Mathieu Pont and Julien Tierny are with the CNRS and Sorbonne Universit\'e.
E-mails: \{firstname.lastname\}@sorbonne-universite.fr
}

%other entries to be set up for journal
\shortauthortitle{Biv \MakeLowercase{\textit{et al.}}: Global Illumination for Fun and Profit}
%\shortauthortitle{Firstauthor \MakeLowercase{\textit{et al.}}: Paper Title}

%% Abstract section.

%% Keywords that describe your work. Will show as 'Index Terms' in journal
%% please capitalize first letter and insert punctuation after last keyword
% \keywords{Topological data analysis, ensemble data, merge trees, persistence diagrams}

%% ACM Computing Classification System (CCS). 
%% See <http://www.acm.org/class/1998/> for details.
%% The ``\CCScat'' command takes four arguments.

% \CCScatlist{ % not used in journal version
%  \CCScat{K.6.1}{Management of Computing and Information Systems}%
% {Project and People Management}{Life Cycle};
%  \CCScat{K.7.m}{The Computing Profession}{Miscellaneous}{Ethics}
% }

%% Uncomment below to include a teaser figure.

%% Uncomment below to disable the manuscript note
%\renewcommand{\manuscriptnotetxt}{}

%% Copyright space is enabled by default as required by guidelines.
%% It is disabled by the 'review' option or via the following command:
% \nocopyrightspace

\vgtcinsertpkg

%%%%%%%%%%%%%%%%%%%%%%%%%%%%%%%%%%%%%%%%%%%%%%%%%%%%%%%%%%%%%%%%
%%%%%%%%%%%%%%%%%%%%%% START OF THE PAPER %%%%%%%%%%%%%%%%%%%%%%
%%%%%%%%%%%%%%%%%%%%%%%%%%%%%%%%%%%%%%%%%%%%%%%%%%%%%%%%%%%%%%%%%

% \newcommand{\axisNotation}[1]{\vectorNotation{#1}}

% \newcommand{\normalizedTree}{N}

% \renewcommand{\julien}[1]{\textcolor{black}{#1}}

\newcommand{\cutout}[1]{\textcolor{blue}{#1}}
\renewcommand{\cutout}[1]{}

\begin{document}

%% The ``\maketitle'' command must be the first command after the
%% ``\begin{document}'' command. It prepares and prints the title block.

%% the only exception to this rule is the \firstsection command

\maketitle

\input{appendixEnergyDerivatives.tex}
\input{appendixPersistenceCorrelation.tex}
\input{appendixMetricDistortion.tex}

%\input(appendixMetricsTable.tex}

%% if specified like this the section will be committed in review mode
\acknowledgments{
The authors wish to thank A, B, and C. This work was supported in part by
a grant from XYZ (\# 12345-67890).}

% \cleardoublepage

%\bibliographystyle{abbrv}
\bibliographystyle{abbrv-doi}

\bibliography{template}
\end{document}
